# Supplementary material for: Knowledge for a warmer world: a patent analysis of climate change adaptation technologies
Source: arXiv:2108.03722 source file (2022-04-21)
Supplement: Supplementary file 1 [file results_supplemented_data.tex]

\FloatBarrier
\section{The scientific knowledge base of adaptation technologies with supplementary information}

\subsection{Overview of CCAT patents}
\begin{figure}
{    \centering
    \includegraphics[width=\textwidth]{inputs_family_based/Piecharts_comparison.pdf}
    \caption{Relative frequencies of different technologies}
    \label{fig:family_based_pie_chart_all}
    }
    \footnotesize
    Notes: These pie charts illustrate the relative frequencies of different types of mitigation and adaptation technologies as counted by patents tagged by the respective CPC code. The figures at the left show pie charts for all Y02-tagged technologies (with adaptation technologies indicated in red color). The figures at the right show these numbers for the subset of adaptation technologies. 
\end{figure}

\begin{landscape}
\input{inputs_supplemented_data/Table_overview_patents_adaptation_family_based_public_gov_support_inventor_type_1976_2017}
\end{landscape}
\input{inputs_supplemented_data/Table_overview_patents_split_adaptation_family_based_public_gov_support_inventor_type_1976_2017}
\begin{landscape}
\input{inputs_supplemented_data/Table_overview_science_citations_adaptation_family_based_public_gov_support_inventor_type_1976_2017}
\end{landscape}

\FloatBarrier
\subsection{Inventive activity in CCAT over time}

\begin{figure}
\caption{Share of adaptation technologies over time}
    \label{fig:timeseries_shares}
\begin{subfigure}{.45\textwidth}
    \centering
    \caption{By technology as share in all patents}
    \label{subfig:ts_share_tech1}
    \includegraphics[width=\textwidth]{inputs_supplemented_data/timeseriese_share_patents/timeseries_Adaptation_share_by_technology.pdf}
\end{subfigure}
\begin{subfigure}{.45\textwidth}
    \centering
    \caption{By technology as share in Y02 patents}
    \label{subfig:ts_share_tech2}
    \includegraphics[width=\textwidth]{inputs_supplemented_data/timeseriese_share_patents/timeseries_Adaptation_share_in_green_patents_by_technology.pdf}
\end{subfigure}

\begin{subfigure}{.45\textwidth}
    \centering
    \caption{Private-public good as share in all patents}
    \label{subfig:ts_share_pubpri1}
    \includegraphics[width=\textwidth]{inputs_supplemented_data/timeseriese_share_patents/timeseries_Adaptation_share_by_public-private_good.pdf}
\end{subfigure}
\begin{subfigure}{.45\textwidth}
    \centering
    \caption{Private-public good as share in Y02 patents}
    \label{subfig:ts_share_pubpri2}
    \includegraphics[width=\textwidth]{inputs_supplemented_data/timeseriese_share_patents/timeseries_Adaptation_share_in_green_patents_by_public-private_good.pdf}
\end{subfigure}

\begin{subfigure}{.45\textwidth}
    \centering
    \caption{By inventor type as share in all patents}
    \label{subfig:ts_share_inv1}
    \includegraphics[width=\textwidth]{inputs_supplemented_data/timeseriese_share_patents/timeseries_Adaptation_share_by_inventor_type.pdf}
\end{subfigure}
\begin{subfigure}{.45\textwidth}
    \centering
    \caption{By inventor type as share in Y02 patents}
    \label{subfig:ts_share_inv2}
    \includegraphics[width=\textwidth]{inputs_supplemented_data/timeseriese_share_patents/timeseries_Adaptation_share_in_green_patents_by_inventor_type.pdf}
\end{subfigure}

\begin{subfigure}{.45\textwidth}
    \centering
    \caption{By public support as share in all patents}
    \label{subfig:ts_share_supp1}
    \includegraphics[width=\textwidth]{inputs_supplemented_data/timeseriese_share_patents/timeseries_Adaptation_share_by_government_support.pdf}
\end{subfigure}
\begin{subfigure}{.45\textwidth}
    \centering
    \caption{By public support as share in Y02 patents}
    \label{subfig:ts_share_supp2}
    \includegraphics[width=\textwidth]{inputs_supplemented_data/timeseriese_share_patents/timeseries_Adaptation_share_in_green_patents_by_government_support.pdf}
\end{subfigure}

    \end{figure}
    
    \begin{figure}
\caption{Share of adaptation technologies over time}
    \label{fig:timeseries_shares_int}

\begin{subfigure}{.45\textwidth}
    \centering
    \caption{Private-public-technology type as share in all patents}
    \label{subfig:ts_share_techpubpri1}
    \includegraphics[width=\textwidth]{inputs_supplemented_data/timeseriese_share_patents/timeseries_Adaptation_share_by_technology_public-private_good.pdf}
\end{subfigure}
\begin{subfigure}{.45\textwidth}
    \centering
    \caption{Private-public-technology type as share in Y02 patents}
    \label{subfig:ts_share_techpubpri2}
    \includegraphics[width=\textwidth]{inputs_supplemented_data/timeseriese_share_patents/timeseries_Adaptation_share_in_green_patents_by_technology_public-private_good.pdf}
\end{subfigure}

\begin{subfigure}{.45\textwidth}
    \centering
    \caption{By technology \& support as share in all patents}
    \label{subfig:ts_share_techsupp1}
    \includegraphics[width=\textwidth]{inputs_supplemented_data/timeseriese_share_patents/timeseries_Adaptation_share_by_technology_government_support.pdf}
\end{subfigure}
\begin{subfigure}{.45\textwidth}
    \centering
    \caption{By technology \& support as share in Y02 patents}
    \label{subfig:ts_share_techsupp2}
    \includegraphics[width=\textwidth]{inputs_supplemented_data/timeseriese_share_patents/timeseries_Adaptation_share_in_green_patents_by_technology_government_support.pdf}
\end{subfigure}

\begin{subfigure}{.45\textwidth}
    \centering
    \caption{By technology \& inventor as share in all patents}
    \label{subfig:ts_share_techinv1}
    \includegraphics[width=\textwidth]{inputs_supplemented_data/timeseriese_share_patents/timeseries_Adaptation_share_by_technology_inventor_type.pdf}
\end{subfigure}
\begin{subfigure}{.45\textwidth}
    \centering
    \caption{By technology \& inventor as share in Y02 patents}
    \label{subfig:ts_share_techinv2}
    \includegraphics[width=\textwidth]{inputs_supplemented_data/timeseriese_share_patents/timeseries_Adaptation_share_in_green_patents_by_technology_inventor_type.pdf}
\end{subfigure}
\end{figure}

\begin{figure}
    \caption{Share of adaptation technologies over time}
    \label{fig:timeseries_shares_int}

\begin{subfigure}{.45\textwidth}
    \centering
    \caption{Private-public-inventor type as share in all patents}
    \label{subfig:ts_share_techpubpri1}
    \includegraphics[width=\textwidth]{inputs_supplemented_data/timeseriese_share_patents/timeseries_Adaptation_share_by_public-private_good_inventor_type.pdf}
\end{subfigure}
\begin{subfigure}{.45\textwidth}
    \centering
    \caption{Private-public-inventor type as share in Y02 patents}
    \label{subfig:ts_share_techpubpri2}
    \includegraphics[width=\textwidth]{inputs_supplemented_data/timeseriese_share_patents/timeseries_Adaptation_share_in_green_patents_by_public-private_good_inventor_type.pdf}
\end{subfigure}

\begin{subfigure}{.45\textwidth}
    \centering
    \caption{Private-public-public support as share in all patents}
    \label{subfig:ts_share_techpubpri1}
    \includegraphics[width=\textwidth]{inputs_supplemented_data/timeseriese_share_patents/timeseries_Adaptation_share_by_public-private_good_government_support.pdf}
\end{subfigure}
\begin{subfigure}{.45\textwidth}
    \centering
    \caption{Private-public-public support as share in Y02 patents}
    \label{subfig:ts_share_techpubpri2}
    \includegraphics[width=\textwidth]{inputs_supplemented_data/timeseriese_share_patents/timeseries_Adaptation_share_in_green_patents_by_public-private_good_government_support.pdf}
\end{subfigure}

\begin{subfigure}{.45\textwidth}
    \centering
    \caption{Inventor type \& public support as share in all patents}
    \label{subfig:ts_share_techpubpri1}
    \includegraphics[width=\textwidth]{inputs_supplemented_data/timeseriese_share_patents/timeseries_Adaptation_share_by_inventor_type_government_support.pdf}
\end{subfigure}
\begin{subfigure}{.45\textwidth}
    \centering
    \caption{Inventor type \& public support as share in Y02 patents}
    \label{subfig:ts_share_techpubpri2}
    \includegraphics[width=\textwidth]{inputs_supplemented_data/timeseriese_share_patents/timeseries_Adaptation_share_in_green_patents_by_inventor_type_government_support.pdf}
\end{subfigure}
\end{figure}

\FloatBarrier

\subsection{Scientificness of CCAT over time}

\begin{figure}
    {\centering
        \caption{CCAT patents and their scientificness over time by technology}
    \label{fig:ts_scientificness_tech}
    \includegraphics[width=\textwidth]{inputs_supplemented_data/timeseriese_scientificness/citingpats_timeseries_Adaptation_by_technology.pdf}
    
    \includegraphics[width=\textwidth]{inputs_supplemented_data/timeseriese_scientificness/scientific_citeshare_Adaptation_by_technology.pdf}
    }
    \footnotesize
    Notes: Upper panel: Number of patents and patents citing to science over time at a logarithmic scale. Lower panel: Science-intensity of patents measures by the share of citations to science in the number of total citations (sum of citations to other patents and scientific articles).  

\end{figure}

\begin{figure}
    {\centering
        \caption{CCAT patents and their scientificness over time by public-private good distinction}
    \label{fig:ts_scientificness_status}
    \includegraphics[width=\textwidth]{inputs_supplemented_data/timeseriese_scientificness/citingpats_timeseries_Adaptation_by_public_private_good.pdf}
    
    \includegraphics[width=\textwidth]{inputs_supplemented_data/timeseriese_scientificness/scientific_citeshare_Adaptation_by_public_private_good.pdf}
    }
    \footnotesize
    Notes: Upper panel: Number of patents and patents citing to science over time at a logarithmic scale. Lower panel: Science-intensity of patents measures by the share of citations to science in the number of total citations (sum of citations to other patents and scientific articles).  

\end{figure}

\begin{figure}
    {\centering
        \caption{CCAT patents and their scientificness over time by inventor type}
    \label{fig:ts_scientificness_status}
    \includegraphics[width=\textwidth]{inputs_supplemented_data/timeseriese_scientificness/citingpats_timeseries_Adaptation_by_inventor_type.pdf}
    
    \includegraphics[width=\textwidth]{inputs_supplemented_data/timeseriese_scientificness/scientific_citeshare_Adaptation_by_inventor_type.pdf}
    }
    \footnotesize
    Notes: Upper panel: Number of patents and patents citing to science over time at a logarithmic scale. Lower panel: Science-intensity of patents measures by the share of citations to science in the number of total citations (sum of citations to other patents and scientific articles).  

\end{figure}

\begin{figure}
    {\centering
        \caption{CCAT patents and their scientificness over time by reliance on government support}
    \label{fig:ts_scientificness_status}
    \includegraphics[width=\textwidth]{inputs_supplemented_data/timeseriese_scientificness/citingpats_timeseries_Adaptation_by_government_support.pdf}
    
    \includegraphics[width=\textwidth]{inputs_supplemented_data/timeseriese_scientificness/scientific_citeshare_Adaptation_by_government_support.pdf}
    }
    \footnotesize
    Notes: Upper panel: Number of patents and patents citing to science over time at a logarithmic scale. Lower panel: Science-intensity of patents measures by the share of citations to science in the number of total citations (sum of citations to other patents and scientific articles).  
\end{figure}

\begin{figure}
    {\centering
        \caption{CCAT patents and their scientificness over time by technology \& public-private good distinction}
    \label{fig:ts_scientificness_status}
    \includegraphics[width=\textwidth]{inputs_supplemented_data/timeseriese_scientificness/citingpats_timeseries_Adaptation_by_technology_public_private_good.pdf}
    
    \includegraphics[width=\textwidth]{inputs_supplemented_data/timeseriese_scientificness/scientific_citeshare_Adaptation_by_technology_public_private_good.pdf}
    }
    \footnotesize
    Notes: Upper panel: Number of patents and patents citing to science over time at a logarithmic scale. Lower panel: Science-intensity of patents measures by the share of citations to science in the number of total citations (sum of citations to other patents and scientific articles).  
\end{figure}

\begin{figure}
    {\centering
        \caption{CCAT patents and their scientificness over time by technology \& inventor}
    \label{fig:ts_scientificness_status}
    
    \includegraphics[width=0.8\textwidth]{inputs_supplemented_data/timeseriese_scientificness/citingpats_timeseries_Adaptation_by_technology_inventor_type.pdf}
    \centering
    \includegraphics[width=0.8\textwidth]{inputs_supplemented_data/timeseriese_scientificness/scientific_citeshare_Adaptation_by_technology_inventor_type.pdf}
    }
    
    \footnotesize
    Notes: Upper panel: Number of patents and patents citing to science over time at a logarithmic scale. Lower panel: Science-intensity of patents measures by the share of citations to science in the number of total citations (sum of citations to other patents and scientific articles).  
\end{figure}

\begin{figure}
    {\centering
        \caption{CCAT patents and their scientificness over time by inventor type \& reliance on government support}
    \label{fig:ts_scientificness_status}
    \includegraphics[width=\textwidth]{inputs_supplemented_data/timeseriese_scientificness/citingpats_timeseries_Adaptation_by_inventor_type_government_support.pdf}
    
    \includegraphics[width=\textwidth]{inputs_supplemented_data/timeseriese_scientificness/scientific_citeshare_Adaptation_by_inventor_type_government_support.pdf}
    }
    \footnotesize
    Notes: Upper panel: Number of patents and patents citing to science over time at a logarithmic scale. Lower panel: Science-intensity of patents measures by the share of citations to science in the number of total citations (sum of citations to other patents and scientific articles).  
\end{figure}

\begin{figure}
    {\centering
        \caption{CCAT patents and their scientificness over time by inventor type \& reliance on government support}
    \label{fig:ts_scientificness_status}
    \includegraphics[width=\textwidth]{inputs_supplemented_data/timeseriese_scientificness/citingpats_timeseries_Adaptation_by_public_private_good_government_support.pdf}
    
    \includegraphics[width=\textwidth]{inputs_supplemented_data/timeseriese_scientificness/scientific_citeshare_Adaptation_by_public_private_good_government_support.pdf}
    }
    \footnotesize
    Notes: Upper panel: Number of patents and patents citing to science over time at a logarithmic scale. Lower panel: Science-intensity of patents measures by the share of citations to science in the number of total citations (sum of citations to other patents and scientific articles).  
\end{figure}

\FloatBarrier

\subsection{The technological and scientific knowledge base of CCAT}
\begin{figure}
{    \centering
    \textbf{Technological similarity by CPC4 citations:} \\
    \includegraphics[width=\textwidth]{inputs_supplemented_data/networks/networks_similarity_CPC4_Adaptation.pdf}
    
    \textbf{Scientific similarity by WoS field citations:} \\
    \includegraphics[width=\textwidth]{inputs_supplemented_data/networks/networks_similarity_WoS_Adaptation.pdf}
    \caption{Cosine similarity networks}
    \label{fig:family_based_similarity_networks_adaptation}
    }
    
    \footnotesize 
    Notes: The networks are based on shares of (a) citations to scientific fields (WoS) and (b) citations to CPC 4-digit technology classes. A link between a pair of adaptation technologies indicates the cosine similarity of their references to scientific fields and technology classes, respectively. For clarity only the strongest two thirds of links are shown. The widths of connecting edges are proportional to the degree of similarity and the node sizes are proportional to the number of patents.
\end{figure}

\begin{figure}
  {  \centering
        \caption{Technological and scientific knowledge base of CCAT by technology type}
    \label{fig:knowledgebase_tech}
    \includegraphics[width=\textwidth]{inputs_supplemented_data/coclasses/Coclassifications_over_time_1_digit_Adaptation_by_technology.pdf}

    \vspace{-1cm}
    
    \includegraphics[width=\textwidth]{inputs_supplemented_data/wosreliance/green_reliance_on_wos_Adaptation_by_technology.pdf}
    
}
\footnotesize
Notes: The technological knowledge base (upper panel) is described by the relative number of co-classifications of CCAT with other CPC classes. The letters indicate technology groups, i.e. A: Human necessities; B: Performing operations \& Transportation; C: Chemistry \& metallurgy; D: Textiles \& paper; E: Fixed constructions; F: Mechanical engineering, lighting, heating, weapons, blasting; G: Physics; H: Electricity; Y: General tagging of new technologies \& technologies spanning over several IPC sections and subjects from former USPC cross-reference sections. The scientific knowledge base (lower panel) is reflected in the field of science (WoS categories) by which scientific articles that are cited by CCAT are classified. 
\end{figure}
\begin{figure}
  {  \centering
        \caption{Technological knowledge base (disaggregate) of CCAT by technology type}
    \label{fig:knowledgebase_tech_disagg}

    \includegraphics[width=\textwidth]{inputs_supplemented_data/coclasses/Coclassifications_over_time_3_digit_Adaptation_by_technology.pdf}
    
    \vspace{1cm}
    
    \includegraphics[width=\textwidth]{inputs_supplemented_data/coclasses/Coclassifications_over_time_4_digit_Adaptation_by_technology.pdf}

}
\footnotesize
Notes: The technological knowledge base is described by the relative number of co-classifications of CCAT with other CPC classes at the 3- and 4-digit level. The letters indicate technology groups, i.e. A: Human necessities; B: Performing operations \& Transportation; C: Chemistry \& metallurgy; D: Textiles \& paper; E: Fixed constructions; F: Mechanical engineering, lighting, heating, weapons, blasting; G: Physics; H: Electricity; Y: General tagging of new technologies \& technologies spanning over several IPC sections and subjects from former USPC cross-reference sections.
\end{figure}

\begin{figure}
  {  \centering
        \caption{Technological and scientific knowledge base of CCAT by public-private good distinction}
    \label{fig:knowledgebase_tech}
    \includegraphics[width=\textwidth]{inputs_supplemented_data/coclasses/Coclassifications_over_time_1_digit_Adaptation_by_public_private_good.pdf}

    \vspace{-1cm}
    
    \includegraphics[width=\textwidth]{inputs_supplemented_data/wosreliance/green_reliance_on_wos_Adaptation_by_public_private_good.pdf}
    
}
\footnotesize
Notes: The technological knowledge base (upper panel) is described by the relative number of co-classifications of CCAT with other CPC classes. The letters indicate technology groups, i.e. A: Human necessities; B: Performing operations \& Transportation; C: Chemistry \& metallurgy; D: Textiles \& paper; E: Fixed constructions; F: Mechanical engineering, lighting, heating, weapons, blasting; G: Physics; H: Electricity; Y: General tagging of new technologies \& technologies spanning over several IPC sections and subjects from former USPC cross-reference sections. The scientific knowledge base (lower panel) is reflected in the field of science (WoS categories) by which scientific articles that are cited by CCAT are classified. 
\end{figure}
\begin{figure}
  {  \centering
        \caption{Technological knowledge base (disaggregate) of CCAT by public-private good distinction}
    \label{fig:knowledgebase_tech_disagg}

    \includegraphics[width=\textwidth]{inputs_supplemented_data/coclasses/Coclassifications_over_time_3_digit_Adaptation_by_public_private_good.pdf}
    
    \vspace{1cm}
    
    \includegraphics[width=\textwidth]{inputs_supplemented_data/coclasses/Coclassifications_over_time_4_digit_Adaptation_by_public_private_good.pdf}

}
\footnotesize
Notes: The technological knowledge base is described by the relative number of co-classifications of CCAT with other CPC classes at the 3- and 4-digit level. The letters indicate technology groups, i.e. A: Human necessities; B: Performing operations \& Transportation; C: Chemistry \& metallurgy; D: Textiles \& paper; E: Fixed constructions; F: Mechanical engineering, lighting, heating, weapons, blasting; G: Physics; H: Electricity; Y: General tagging of new technologies \& technologies spanning over several IPC sections and subjects from former USPC cross-reference sections.
\end{figure}

\begin{figure}
  {  \centering
        \caption{Technological and scientific knowledge base of CCAT by inventor type}
    \label{fig:knowledgebase_tech}
    \includegraphics[width=\textwidth]{inputs_supplemented_data/coclasses/Coclassifications_over_time_1_digit_Adaptation_by_inventor_type.pdf}

    \vspace{-1cm}
    
    \includegraphics[width=\textwidth]{inputs_supplemented_data/wosreliance/green_reliance_on_wos_Adaptation_by_inventor_type.pdf}
    
}
\footnotesize
Notes: The technological knowledge base (upper panel) is described by the relative number of co-classifications of CCAT with other CPC classes. The letters indicate technology groups, i.e. A: Human necessities; B: Performing operations \& Transportation; C: Chemistry \& metallurgy; D: Textiles \& paper; E: Fixed constructions; F: Mechanical engineering, lighting, heating, weapons, blasting; G: Physics; H: Electricity; Y: General tagging of new technologies \& technologies spanning over several IPC sections and subjects from former USPC cross-reference sections. The scientific knowledge base (lower panel) is reflected in the field of science (WoS categories) by which scientific articles that are cited by CCAT are classified. 
\end{figure}
\begin{figure}
  {  \centering
        \caption{Technological knowledge base (disaggregate) of CCAT by inventor type}
    \label{fig:knowledgebase_tech_disagg}

    \includegraphics[width=\textwidth]{inputs_supplemented_data/coclasses/Coclassifications_over_time_3_digit_Adaptation_by_inventor_type.pdf}
    
    \vspace{1cm}
    
    \includegraphics[width=\textwidth]{inputs_supplemented_data/coclasses/Coclassifications_over_time_4_digit_Adaptation_by_inventor_type.pdf}

}
\footnotesize
Notes: The technological knowledge base is described by the relative number of co-classifications of CCAT with other CPC classes at the 3- and 4-digit level. The letters indicate technology groups, i.e. A: Human necessities; B: Performing operations \& Transportation; C: Chemistry \& metallurgy; D: Textiles \& paper; E: Fixed constructions; F: Mechanical engineering, lighting, heating, weapons, blasting; G: Physics; H: Electricity; Y: General tagging of new technologies \& technologies spanning over several IPC sections and subjects from former USPC cross-reference sections.
\end{figure}

\begin{figure}
  {  \centering
        \caption{Technological and scientific knowledge base of CCAT by reliance on government support}
    \label{fig:knowledgebase_tech}
    \includegraphics[width=\textwidth]{inputs_supplemented_data/coclasses/Coclassifications_over_time_1_digit_Adaptation_by_government_support.pdf}

    \vspace{-1cm}
    
    \includegraphics[width=\textwidth]{inputs_supplemented_data/wosreliance/green_reliance_on_wos_Adaptation_by_government_support.pdf}
    
}
\footnotesize
Notes: The technological knowledge base (upper panel) is described by the relative number of co-classifications of CCAT with other CPC classes. The letters indicate technology groups, i.e. A: Human necessities; B: Performing operations \& Transportation; C: Chemistry \& metallurgy; D: Textiles \& paper; E: Fixed constructions; F: Mechanical engineering, lighting, heating, weapons, blasting; G: Physics; H: Electricity; Y: General tagging of new technologies \& technologies spanning over several IPC sections and subjects from former USPC cross-reference sections. The scientific knowledge base (lower panel) is reflected in the field of science (WoS categories) by which scientific articles that are cited by CCAT are classified. 
\end{figure}
\begin{figure}
  {  \centering
        \caption{Technological knowledge base (disaggregate) of CCAT by reliance on government support}
    \label{fig:knowledgebase_tech_disagg}

    \includegraphics[width=\textwidth]{inputs_supplemented_data/coclasses/Coclassifications_over_time_3_digit_Adaptation_by_government_support.pdf}
    
    \vspace{1cm}
    
    \includegraphics[width=\textwidth]{inputs_supplemented_data/coclasses/Coclassifications_over_time_4_digit_Adaptation_by_government_support.pdf}

}
\footnotesize
Notes: The technological knowledge base is described by the relative number of co-classifications of CCAT with other CPC classes at the 3- and 4-digit level. The letters indicate technology groups, i.e. A: Human necessities; B: Performing operations \& Transportation; C: Chemistry \& metallurgy; D: Textiles \& paper; E: Fixed constructions; F: Mechanical engineering, lighting, heating, weapons, blasting; G: Physics; H: Electricity; Y: General tagging of new technologies \& technologies spanning over several IPC sections and subjects from former USPC cross-reference sections.
\end{figure}

\begin{figure}
  {  \centering
        \caption{Technological and scientific knowledge base of CCAT by technology \& public-private good distinction}
    \label{fig:knowledgebase_tech}
    \includegraphics[width=\textwidth]{inputs_supplemented_data/coclasses/Coclassifications_over_time_1_digit_Adaptation_by_technology_public_private_good.pdf}

    \vspace{-1cm}
    
    \includegraphics[width=\textwidth]{inputs_supplemented_data/wosreliance/green_reliance_on_wos_Adaptation_by_technology_public_private_good.pdf}
    
}
\footnotesize
Notes: The technological knowledge base (upper panel) is described by the relative number of co-classifications of CCAT with other CPC classes. The letters indicate technology groups, i.e. A: Human necessities; B: Performing operations \& Transportation; C: Chemistry \& metallurgy; D: Textiles \& paper; E: Fixed constructions; F: Mechanical engineering, lighting, heating, weapons, blasting; G: Physics; H: Electricity; Y: General tagging of new technologies \& technologies spanning over several IPC sections and subjects from former USPC cross-reference sections. The scientific knowledge base (lower panel) is reflected in the field of science (WoS categories) by which scientific articles that are cited by CCAT are classified. 
\end{figure}
\begin{figure}
  {  \centering
        \caption{Technological knowledge base (disaggregate) of CCAT by technology \& public-private good distinction}
    \label{fig:knowledgebase_tech_disagg}

    \includegraphics[width=\textwidth]{inputs_supplemented_data/coclasses/Coclassifications_over_time_3_digit_Adaptation_by_technology_public_private_good.pdf}
    
    \vspace{1cm}
    
    \includegraphics[width=\textwidth]{inputs_supplemented_data/coclasses/Coclassifications_over_time_4_digit_Adaptation_by_technology_public_private_good.pdf}

}
\footnotesize
Notes: The technological knowledge base is described by the relative number of co-classifications of CCAT with other CPC classes at the 3- and 4-digit level. The letters indicate technology groups, i.e. A: Human necessities; B: Performing operations \& Transportation; C: Chemistry \& metallurgy; D: Textiles \& paper; E: Fixed constructions; F: Mechanical engineering, lighting, heating, weapons, blasting; G: Physics; H: Electricity; Y: General tagging of new technologies \& technologies spanning over several IPC sections and subjects from former USPC cross-reference sections.
\end{figure}

\begin{figure}
  {  \centering
        \caption{Technological and scientific knowledge base of CCAT by technology \& inventor type}
    \label{fig:knowledgebase_tech}
    \includegraphics[width=\textwidth]{inputs_supplemented_data/coclasses/Coclassifications_over_time_1_digit_Adaptation_by_technology_inventor_type.pdf}

    \vspace{-1cm}
    
    \includegraphics[width=\textwidth]{inputs_supplemented_data/wosreliance/green_reliance_on_wos_Adaptation_by_technology_inventor_type.pdf}
    
}
\footnotesize
Notes: The technological knowledge base (upper panel) is described by the relative number of co-classifications of CCAT with other CPC classes. The letters indicate technology groups, i.e. A: Human necessities; B: Performing operations \& Transportation; C: Chemistry \& metallurgy; D: Textiles \& paper; E: Fixed constructions; F: Mechanical engineering, lighting, heating, weapons, blasting; G: Physics; H: Electricity; Y: General tagging of new technologies \& technologies spanning over several IPC sections and subjects from former USPC cross-reference sections. The scientific knowledge base (lower panel) is reflected in the field of science (WoS categories) by which scientific articles that are cited by CCAT are classified. 
\end{figure}
\begin{figure}
  {  \centering
        \caption{Technological knowledge base (disaggregate) of CCAT by technology \& inventor type}
    \label{fig:knowledgebase_tech_disagg}

    \includegraphics[width=\textwidth]{inputs_supplemented_data/coclasses/Coclassifications_over_time_3_digit_Adaptation_by_technology_inventor_type.pdf}
    
    \vspace{1cm}
    
    \includegraphics[width=\textwidth]{inputs_supplemented_data/coclasses/Coclassifications_over_time_4_digit_Adaptation_by_technology_inventor_type.pdf}

}
\footnotesize
Notes: The technological knowledge base is described by the relative number of co-classifications of CCAT with other CPC classes at the 3- and 4-digit level. The letters indicate technology groups, i.e. A: Human necessities; B: Performing operations \& Transportation; C: Chemistry \& metallurgy; D: Textiles \& paper; E: Fixed constructions; F: Mechanical engineering, lighting, heating, weapons, blasting; G: Physics; H: Electricity; Y: General tagging of new technologies \& technologies spanning over several IPC sections and subjects from former USPC cross-reference sections.
\end{figure}

\begin{figure}
  {  \centering
        \caption{Technological and scientific knowledge base of CCAT by technology \& reliance on government support}
    \label{fig:knowledgebase_tech}
    \includegraphics[width=\textwidth]{inputs_supplemented_data/coclasses/Coclassifications_over_time_1_digit_Adaptation_by_technology_government_support.pdf}

    \vspace{-1cm}
    
    \includegraphics[width=\textwidth]{inputs_supplemented_data/wosreliance/green_reliance_on_wos_Adaptation_by_technology_public_private_good.pdf}
    
}
\footnotesize
Notes: The technological knowledge base (upper panel) is described by the relative number of co-classifications of CCAT with other CPC classes. The letters indicate technology groups, i.e. A: Human necessities; B: Performing operations \& Transportation; C: Chemistry \& metallurgy; D: Textiles \& paper; E: Fixed constructions; F: Mechanical engineering, lighting, heating, weapons, blasting; G: Physics; H: Electricity; Y: General tagging of new technologies \& technologies spanning over several IPC sections and subjects from former USPC cross-reference sections. The scientific knowledge base (lower panel) is reflected in the field of science (WoS categories) by which scientific articles that are cited by CCAT are classified. 
\end{figure}
\begin{figure}
  {  \centering
        \caption{Technological knowledge base (disaggregate) of CCAT by technology \& public-private good distinction}
    \label{fig:knowledgebase_tech_disagg}

    \includegraphics[width=\textwidth]{inputs_supplemented_data/coclasses/Coclassifications_over_time_3_digit_Adaptation_by_technology_public_private_good.pdf}
    
    \vspace{1cm}
    
    \includegraphics[width=\textwidth]{inputs_supplemented_data/coclasses/Coclassifications_over_time_4_digit_Adaptation_by_technology_public_private_good.pdf}

}
\footnotesize
Notes: The technological knowledge base is described by the relative number of co-classifications of CCAT with other CPC classes at the 3- and 4-digit level. The letters indicate technology groups, i.e. A: Human necessities; B: Performing operations \& Transportation; C: Chemistry \& metallurgy; D: Textiles \& paper; E: Fixed constructions; F: Mechanical engineering, lighting, heating, weapons, blasting; G: Physics; H: Electricity; Y: General tagging of new technologies \& technologies spanning over several IPC sections and subjects from former USPC cross-reference sections.
\end{figure}

\begin{figure}
  {  \centering
        \caption{Technological and scientific knowledge base of CCAT by technology \& reliance on government support}
    \label{fig:knowledgebase_tech}
    \includegraphics[width=\textwidth]{inputs_supplemented_data/coclasses/Coclassifications_over_time_1_digit_Adaptation_by_technology_government_support.pdf}

    \vspace{-1cm}
    
    \includegraphics[width=\textwidth]{inputs_supplemented_data/wosreliance/green_reliance_on_wos_Adaptation_by_technology_government_support.pdf}
    
}
\footnotesize
Notes: The technological knowledge base (upper panel) is described by the relative number of co-classifications of CCAT with other CPC classes. The letters indicate technology groups, i.e. A: Human necessities; B: Performing operations \& Transportation; C: Chemistry \& metallurgy; D: Textiles \& paper; E: Fixed constructions; F: Mechanical engineering, lighting, heating, weapons, blasting; G: Physics; H: Electricity; Y: General tagging of new technologies \& technologies spanning over several IPC sections and subjects from former USPC cross-reference sections. The scientific knowledge base (lower panel) is reflected in the field of science (WoS categories) by which scientific articles that are cited by CCAT are classified. 
\end{figure}
\begin{figure}
  {  \centering
        \caption{Technological knowledge base (disaggregate) of CCAT by technology \& reliance on government support}
    \label{fig:knowledgebase_tech_disagg}

    \includegraphics[width=\textwidth]{inputs_supplemented_data/coclasses/Coclassifications_over_time_3_digit_Adaptation_by_public_private_good_government_support.pdf}
    
    \vspace{1cm}
    
    \includegraphics[width=\textwidth]{inputs_supplemented_data/coclasses/Coclassifications_over_time_4_digit_Adaptation_by_public_private_good_government_support.pdf}

}
\footnotesize
Notes: The technological knowledge base is described by the relative number of co-classifications of CCAT with other CPC classes at the 3- and 4-digit level. The letters indicate technology groups, i.e. A: Human necessities; B: Performing operations \& Transportation; C: Chemistry \& metallurgy; D: Textiles \& paper; E: Fixed constructions; F: Mechanical engineering, lighting, heating, weapons, blasting; G: Physics; H: Electricity; Y: General tagging of new technologies \& technologies spanning over several IPC sections and subjects from former USPC cross-reference sections.
\end{figure}

\begin{figure}
  {  \centering
        \caption{Technological and scientific knowledge base of CCAT by inventor \& public-private good distinction}
    \label{fig:knowledgebase_tech}
    \includegraphics[width=\textwidth]{inputs_supplemented_data/coclasses/Coclassifications_over_time_1_digit_Adaptation_by_public_private_good_inventor_type.pdf}

    \vspace{-1cm}
    
    \includegraphics[width=\textwidth]{inputs_supplemented_data/wosreliance/green_reliance_on_wos_Adaptation_by_public_private_good_inventor_type.pdf}
    
}
\footnotesize
Notes: The technological knowledge base (upper panel) is described by the relative number of co-classifications of CCAT with other CPC classes. The letters indicate technology groups, i.e. A: Human necessities; B: Performing operations \& Transportation; C: Chemistry \& metallurgy; D: Textiles \& paper; E: Fixed constructions; F: Mechanical engineering, lighting, heating, weapons, blasting; G: Physics; H: Electricity; Y: General tagging of new technologies \& technologies spanning over several IPC sections and subjects from former USPC cross-reference sections. The scientific knowledge base (lower panel) is reflected in the field of science (WoS categories) by which scientific articles that are cited by CCAT are classified. 
\end{figure}
\begin{figure}
  {  \centering
        \caption{Technological knowledge base (disaggregate) of CCAT by inventor \& public-private good distinction}
    \label{fig:knowledgebase_tech_disagg}

    \includegraphics[width=\textwidth]{inputs_supplemented_data/coclasses/Coclassifications_over_time_3_digit_Adaptation_by_public_private_good_government_support.pdf}
    
    \vspace{1cm}
    
    \includegraphics[width=\textwidth]{inputs_supplemented_data/coclasses/Coclassifications_over_time_4_digit_Adaptation_by_public_private_good_government_support.pdf}

}
\footnotesize
Notes: The technological knowledge base is described by the relative number of co-classifications of CCAT with other CPC classes at the 3- and 4-digit level. The letters indicate technology groups, i.e. A: Human necessities; B: Performing operations \& Transportation; C: Chemistry \& metallurgy; D: Textiles \& paper; E: Fixed constructions; F: Mechanical engineering, lighting, heating, weapons, blasting; G: Physics; H: Electricity; Y: General tagging of new technologies \& technologies spanning over several IPC sections and subjects from former USPC cross-reference sections.
\end{figure}

\begin{figure}
  {  \centering
        \caption{Technological and scientific knowledge base of CCAT by inventor \& reliance on government support}
    \label{fig:knowledgebase_tech}
    \includegraphics[width=\textwidth]{inputs_supplemented_data/coclasses/Coclassifications_over_time_1_digit_Adaptation_by_inventor_type_government_support.pdf}

    \vspace{-1cm}
    
    \includegraphics[width=\textwidth]{inputs_supplemented_data/wosreliance/green_reliance_on_wos_Adaptation_by_inventor_type_government_support.pdf}
    
}
\footnotesize
Notes: The technological knowledge base (upper panel) is described by the relative number of co-classifications of CCAT with other CPC classes. The letters indicate technology groups, i.e. A: Human necessities; B: Performing operations \& Transportation; C: Chemistry \& metallurgy; D: Textiles \& paper; E: Fixed constructions; F: Mechanical engineering, lighting, heating, weapons, blasting; G: Physics; H: Electricity; Y: General tagging of new technologies \& technologies spanning over several IPC sections and subjects from former USPC cross-reference sections. The scientific knowledge base (lower panel) is reflected in the field of science (WoS categories) by which scientific articles that are cited by CCAT are classified. 
\end{figure}
\begin{figure}
  {  \centering
        \caption{Technological knowledge base (disaggregate) of CCAT by inventor \& reliance on government support}
    \label{fig:knowledgebase_tech_disagg}

    \includegraphics[width=\textwidth]{inputs_supplemented_data/coclasses/Coclassifications_over_time_3_digit_Adaptation_by_inventor_type_government_support.pdf}
    
    \vspace{1cm}
    
    \includegraphics[width=\textwidth]{inputs_supplemented_data/coclasses/Coclassifications_over_time_4_digit_Adaptation_by_inventor_type_government_support.pdf}

}
\footnotesize
Notes: The technological knowledge base is described by the relative number of co-classifications of CCAT with other CPC classes at the 3- and 4-digit level. The letters indicate technology groups, i.e. A: Human necessities; B: Performing operations \& Transportation; C: Chemistry \& metallurgy; D: Textiles \& paper; E: Fixed constructions; F: Mechanical engineering, lighting, heating, weapons, blasting; G: Physics; H: Electricity; Y: General tagging of new technologies \& technologies spanning over several IPC sections and subjects from former USPC cross-reference sections.
\end{figure}

\begin{figure}
  {  \centering
        \caption{Technological and scientific knowledge base of CCAT by inventor \& reliance on government support}
    \label{fig:knowledgebase_tech}
    \includegraphics[width=\textwidth]{inputs_supplemented_data/coclasses/Coclassifications_over_time_1_digit_Adaptation_by_public_private_good_government_support.pdf}

    \vspace{-1cm}
    
    \includegraphics[width=\textwidth]{inputs_supplemented_data/wosreliance/green_reliance_on_wos_Adaptation_by_public_private_good_government_support.pdf}
    
}
\footnotesize
Notes: The technological knowledge base (upper panel) is described by the relative number of co-classifications of CCAT with other CPC classes. The letters indicate technology groups, i.e. A: Human necessities; B: Performing operations \& Transportation; C: Chemistry \& metallurgy; D: Textiles \& paper; E: Fixed constructions; F: Mechanical engineering, lighting, heating, weapons, blasting; G: Physics; H: Electricity; Y: General tagging of new technologies \& technologies spanning over several IPC sections and subjects from former USPC cross-reference sections. The scientific knowledge base (lower panel) is reflected in the field of science (WoS categories) by which scientific articles that are cited by CCAT are classified. 
\end{figure}
\begin{figure}
  {  \centering
        \caption{Technological knowledge base (disaggregate) of CCAT by inventor \& reliance on government support}
    \label{fig:knowledgebase_tech_disagg}

    \includegraphics[width=\textwidth]{inputs_supplemented_data/coclasses/Coclassifications_over_time_3_digit_Adaptation_by_public_private_good_government_support.pdf}
    
    \vspace{1cm}
    
    \includegraphics[width=\textwidth]{inputs_supplemented_data/coclasses/Coclassifications_over_time_4_digit_Adaptation_by_public_private_good_government_support.pdf}

}
\footnotesize
Notes: The technological knowledge base is described by the relative number of co-classifications of CCAT with other CPC classes at the 3- and 4-digit level. The letters indicate technology groups, i.e. A: Human necessities; B: Performing operations \& Transportation; C: Chemistry \& metallurgy; D: Textiles \& paper; E: Fixed constructions; F: Mechanical engineering, lighting, heating, weapons, blasting; G: Physics; H: Electricity; Y: General tagging of new technologies \& technologies spanning over several IPC sections and subjects from former USPC cross-reference sections.
\end{figure}

\FloatBarrier
\subsubsection{Background information on the science reliance of CCAT}
\input{inputs_supplemented_data/Table_overview_age_adaptation_family_based_public_gov_support_inventor_type_1976_2017}

\input{inputs_supplemented_data/Table_top_citing_patents_adaptation_family_based_public_gov_support_inventor_type_1976_2017}

\input{inputs_supplemented_data/Table_top_WoS_fields_adaptation_family_based_public_gov_support_inventor_type_1976_2017}

\input{inputs_supplemented_data/Table_top_journals_adaptation_family_based_public_gov_support_inventor_type_1976_2017}

\input{inputs_supplemented_data/Table_top_papers_adaptation_family_based_public_gov_support_inventor_type_1976_2017}

\begin{figure}%{!t]
{\centering
\includegraphics[trim = {.8cm 0cm .8cm 0cm}, clip,width=.43\textwidth]{inputs_family_based/science_reliance_change_coastal.pdf}
\includegraphics[trim = {.8cm 0cm .8cm 0cm}, clip,width=.43\textwidth]{inputs_family_based/science_reliance_change_water.pdf}
\includegraphics[trim = {.8cm 0cm .8cm 0cm}, clip,width=.43\textwidth]{inputs_family_based/science_reliance_change_infrastructure.pdf}
\includegraphics[trim = {.8cm 0cm .8cm 0cm}, clip,width=.43\textwidth]{inputs_family_based/science_reliance_change_agriculture.pdf}
\includegraphics[trim = {.8cm 0cm .8cm 0cm}, clip,width=.43\textwidth]{inputs_family_based/science_reliance_change_health.pdf}
\includegraphics[trim = {.8cm 0cm .8cm 0cm}, clip,width=.43\textwidth]{inputs_family_based/science_reliance_change_indirect_adaptation.pdf}
    \caption{Most important scientific fields}
    \label{fig:family_based_SI_science_reliance_change}
    }
    \footnotesize
    Notes: These panels show the ten most important scientific fields per adaptation technology measured as shares of total references citing the field. Scientific fields are ordered from the most to least important field of the most recent time period. (Remark: This figure has the same information as Fig. \ref{fig:wos_fields_adaptation}. We used this style in the Suppl. Material of \cite{hotte2021rise} to show more fields than in Fig. \ref{fig:wos_fields_adaptation}.
\end{figure}
\FloatBarrier
\subsubsection{Technological relatedness with other green technologies}
\begin{figure}
{    \centering
    \textbf{Technological similarity by CPC4 citations:} \\
    \includegraphics[width=\textwidth]{inputs_supplemented_data/networks/networks_similarity_CPC4_all.pdf}
    
    \textbf{Scientific similarity by WoS field citations:} \\
    \includegraphics[width=\textwidth]{inputs_supplemented_data/networks/networks_similarity_WoS_all.pdf}
    \caption{Cosine similarity networks}
    \label{fig:family_based_similarity_networks_adaptation}
    }
    
    \footnotesize 
    Notes: The networks are based on shares of (a) citations to scientific fields (WoS) and (b) citations to CPC 4-digit technology classes. A link between a pair of adaptation technologies indicates the cosine similarity of their references to scientific fields and technology classes, respectively. For clarity only the strongest two thirds of links are shown. The widths of connecting edges are proportional to the degree of similarity and the node sizes are proportional to the number of patents.
\end{figure}

\newpage
\FloatBarrier
